# Supplementary material for: Quantum cellular automata for word statistics facilitated by quantum correlations
Source: arXiv:2504.14453 source file (2025-04-20)
Supplement: Supplementary file 1 [file supp.pdf]

# Supplemental Material: Quantum cellular automata for word statistics facilitated by quantum correlations


Guanhua Chen[1] and Yao Yao[1,2a1]

[11] *Department of Physics, South China University of Technology, Guangzhou 510640, China*
[2] *State Key Laboratory of Luminescent Materials and Devices, South China University of Technology, Guangzhou 510640, China*



(Dated: March 8, 2025)


## I. A MORE COMPLEX CORPUS STATE

In the main text we have discussed a simple corpus state (CS) with three words 'you', 'are' and 'here' to describe the algorithm. Here we provide a more complex example with seven words to clarify how to obtain the CS in the 2-gram model. The pregiven seven words are $\{\mathsf{you}, \mathsf{we}, \mathsf{I}, \mathsf{are}, \mathsf{am}, \mathsf{winners}, \mathsf{a\ winner}\}$ ('a winner' is regarded as a whole word for simplicity) and the physical dimension is $d = 7$. The corpus is consisted of four sentences as shown in the figure below. The resulted CS is a two-site entangled state as

$$
\begin{aligned}
|\mathrm{CS}\rangle &= \sum_{\text{pair}} |\mathsf{word}_1\rangle|\mathsf{word}_2\rangle \\
&= (2|\mathsf{you}\rangle|\mathsf{are}\rangle + 2|\mathsf{are}\rangle|\mathsf{winners}\rangle + |\mathsf{we}\rangle|\mathsf{are}\rangle + |\mathsf{I}\rangle|\mathsf{am}\rangle + |\mathsf{are}\rangle|\mathsf{a\ winner}\rangle + |\mathsf{am}\rangle|\mathsf{a\ winner}\rangle)/\sqrt{12}.
\end{aligned}
\tag{1}
$$

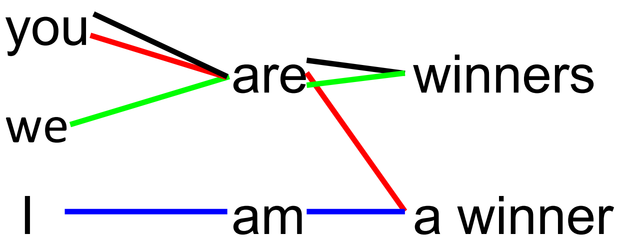


FIG. 1. Four grammatically correct sentences are denoted with different colors of lines which connect word pairs.

## II. THREE-WORD ENTANGLEMENT ASYMMETRY

The entanglement asymmetry (EA) is used to quantify the block-diagonal process of density matrix. In this section, EA of three words $\Delta S^{\mathsf{word}}_{j,j+1}$ are represented in more detail.

We have already known that for any two adjacent sites, $\Delta S^{\mathsf{word}}_{j,j+1} = S(\rho_{j,j+1}) - S(\rho_{j,j+1;\mathsf{word}})$, where $\rho_{j,j+1}$ is the two-site reduced density matrix. $\rho_{j,j+1;\mathsf{word}} = \sum_q \Pi^{\mathsf{word}}_q \rho_{j,j+1} \Pi^{\mathsf{word}}_q$ can be obtained through the projection onto the sector $q$ in the two-site subsystem. Setting the there-level basis of words as

$$
|\mathsf{you}\rangle = \begin{pmatrix}1\\0\\0\end{pmatrix},\ |\mathsf{are}\rangle = \begin{pmatrix}0\\1\\0\end{pmatrix},\ |\mathsf{here}\rangle = \begin{pmatrix}0\\0\\1\end{pmatrix},
\tag{2}
$$

and occupation $N^{\mathsf{word}} = |\mathsf{word}\rangle\langle\mathsf{word}|$. For two sites, charge sector has three choices $q = 0, 1, 2$. Take $|\mathsf{you}\rangle$ as an example, the resulting projectors are

$$
\begin{aligned}
\Pi^{\mathsf{you}}_2 =& N^{\mathsf{you}} \otimes N^{\mathsf{you}} \\
=& \mathrm{diag}(1, 0, 0, 0, 0, 0, 0, 0, 0),
\end{aligned}
\tag{3}
$$


[a] Electronic address: yaoyao2016@scut.edu.cn

$$
\begin{aligned}
\Pi_1^{\mathsf{you}} =& N^{\mathsf{you}} \otimes N^{\mathsf{are}} + N^{\mathsf{you}} \otimes N^{\mathsf{here}} + N^{\mathsf{are}} \otimes N^{\mathsf{you}} + N^{\mathsf{here}} \otimes N^{\mathsf{you}} \\
=& \mathrm{diag}(0,1,1,1,0,0,1,0,0),
\end{aligned} \tag{4}
$$

$$
\begin{aligned}
\Pi_0^{\mathsf{you}} =& N^{\mathsf{are}} \otimes N^{\mathsf{are}} + N^{\mathsf{here}} \otimes N^{\mathsf{here}} + N^{\mathsf{are}} \otimes N^{\mathsf{here}} + N^{\mathsf{here}} \otimes N^{\mathsf{are}} \\
=& \mathrm{diag}(0,0,0,0,1,1,0,1,1),
\end{aligned} \tag{5}
$$

which generate the block-diagonal density matrix.

## III. EVOLUTION OF FROBENIUS DISTANCE

In the figure below we provide additional numerical results of Frobenius distance $D$ which are not displayed in the main text.

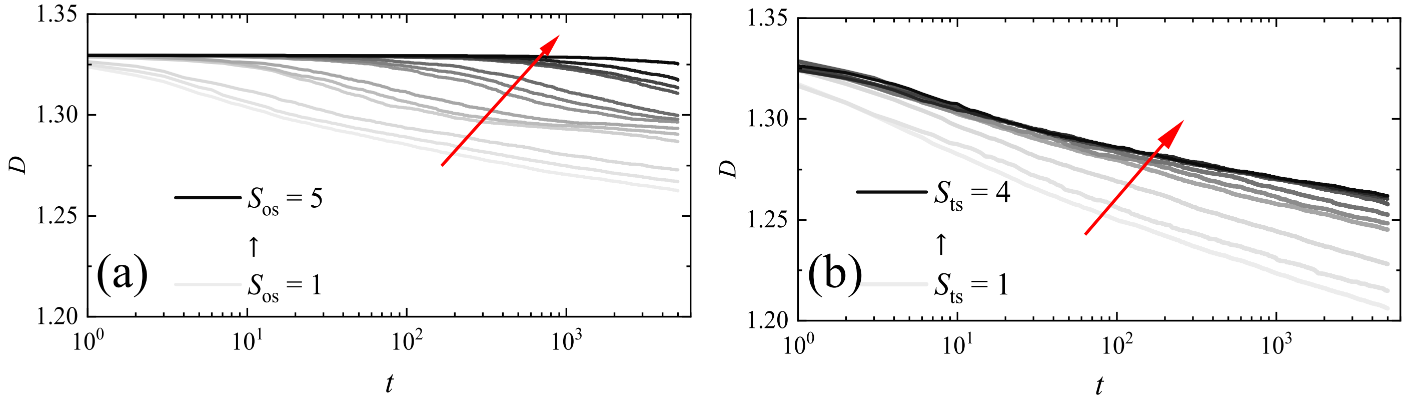


FIG. 2. Evolution of Frobenius distance $D$ with chain $L = 6$ under growing gate entropy (a) $S_{\mathrm{os}}$ without effective two-site gates, (b) $S_{\mathrm{ts}}$ with fixed $S_{\mathrm{os}} = 1$. Red arrows denote the variation trend of curves. These gate entropies are selected from the FIG.3 in the main text every three points.
